# Supplementary material for: Design of two-dimensional particle assemblies using isotropic pair interactions with an attractive well
Source: arXiv:1711.01307 source file (2017-11-03)
Supplement: Supplementary file 1 [file rel_entropy_gams_supp.pdf]

# Supplemental Material

## I. SPECIAL LATTICE COMPETITORS FOR HONEYCOMB AND KAGOME GROUND STATE DESIGN TARGETS

As discussed in the Methods section of the main paper, we illustrate special honeycomb and kagome competitors that emerged during the optimization process in figures S1 and S2 below.

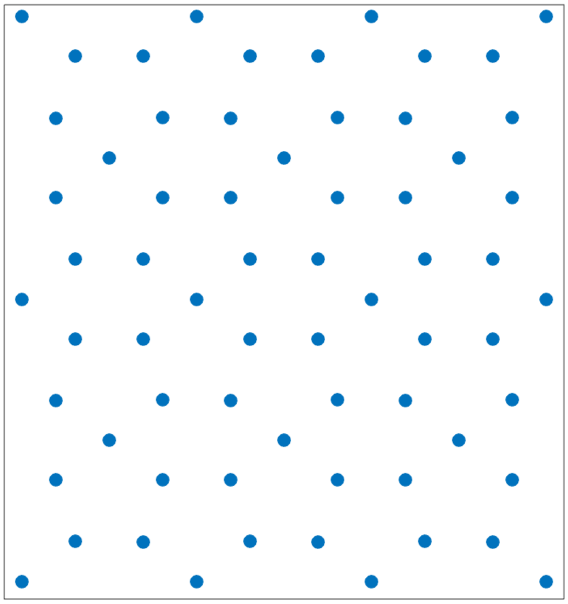

FIG. S1. Special competitor for the design of the honeycomb lattice target. Note that this crystal can be characterized as rows of elongated triangular motifs staggered so as to create intermediate 'pentagonal' motifs between them.

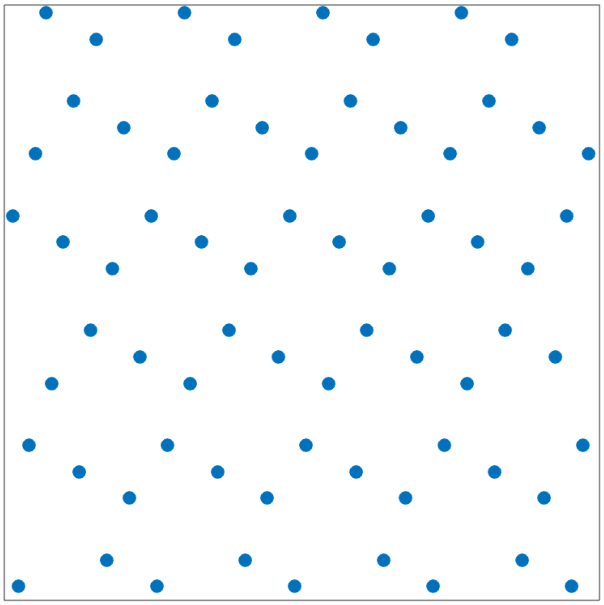

FIG. S2. Special competitor for the design of the kagome lattice target. This crystal resembles a bricked pattern with particles positioned at the outline of each 'brick'. Note further that the 'brick' rows can be related naturally to a kagome lattice row by orthogonalizing the cell from its usual $60^{\rm o}$ inclination

## II. PAIR POTENTIAL PARAMETERS OPTIMIZED FOR THE SQUARE, HONEYCOMB AND KAGOME LATTICES FROM THE GROUND STATE METHOD

We list the potential parameters of $\phi(r)$ (see eq. 1 in main paper) that maximize the stability (as described in the main text) of the square, honeycomb and kagome crystal structures. These are listed separately as the parameters of the soft repulsive component, the cut off radius and the coefficients of the quadratic components of $f_{\rm shift}$ in S1. The second table S2 lists the values of $B_i, r_i, \sigma_i$ in the exp expressions.

TABLE S1. Parameters $A, n, \sigma_0, r_{\text{cut}}$ and $P, Q, R$ for the convex repulsive pair potential $\phi(r)$ found to favor square, honeycomb and kagome respectively at density $\rho = 1.22$. Minimum positions $r_{\text{min}}$ were fixed at 0.905357,1.375846,1.685060 for square, honeycomb and kagome corresponding to the first, second and third coordination shell for each lattice respectively.

| | $A$ | $n$ | $\sigma_0$ | $r_{\text{cut}}$ | $P$ | $Q$ | $R$ |
|---|---|---|---|---|---|---|---|
| Square | 2.50683 | 16.192980 | 0.457063 | 1.4624765 | -12.072094 | 35.164883 | -21.599134 |
| Honeycomb | $7.28842\times10^{-3}$ | 20.071347 | 1.105417 | 1.5152092 | 16.990788 | -45.967663 | 33.479133 |
| Kagome | 1.12196 | 8.8883046 | 0.379738 | 1.9960410 | 18.270237 | -75.490356 | 78.041919 |

TABLE S2. Parameters $B_i, r_i, \sigma_i$ for the convex repulsive pair potential $\phi(r)$ found to favor square, honeycomb and kagome.

| | $B_1$ | $r_1$ | $\sigma_1$ | $B_2$ | $r_2$ | $\sigma_2$ |
|---|---|---|---|---|---|---|
| Square | -4.308569 | 1.376916 | 0.472360 | 0.245501 | 1.417995 | 0.0685170 |
| Honeycomb | -4.290190 | 1.901628 | 0.598765 | -1.432023 | 1.368413 | 0.0645997 |
| Kagome | -4.389501 | 1.595781 | 0.218255 | 0.07949805 | 1.311123 | 0.1323579 |

## III. BINARY MIXTURE COMPETITOR FORWARD CALCULATION FORMULATION

Binary mixture competitor calculation follows directly from a basic treatment of binary phase equilibrium and solved numerically by means of the mathemetical software GAMS. Briefly, we consider a box of constant volume ($V$), particles ($N$) and temperature ($T$). In this canonical ensemble the system may spontaneously phase separate so as to lower the overall system free energy. For our crystal design process, we consider two crystals $l_1$ and $l_2$ at respective densities $\rho_1 = N_1/V_1$ and $\rho_2 = N_2/V_2$ inside a box of total volume $V$ and number of particles $N$ (i.e. system density $\rho = N/V$) co-existing in some relative molar fraction $x_2 = N_2/N$ and $x = 1 - x_2$. Since both crystals must occupy the entire box and conserve the total number of particles we can relate $x$ to $\rho$, $\rho_1$ and $\rho_2$ as

$$(1 - x) = \frac{1/\rho - 1/\rho_1}{1/\rho_2 - 1/\rho_1} \tag{S1}$$

Next, for two phases to co-exist, the common tangent condition states that they must be at equal pressure and chemical potential. This means that

$$P_1 = P_2 \tag{S2}$$

and

$$U_1 + P_1/\rho_1 = U_2 + P_2/\rho_2 \tag{S3}$$

where $U_i$ and $P_i$ denote energies and pressures for each crystal $l_1$ and $l_2$ respectively. Both of these quantities are computed from standard expressions and the energy is given by

$$U_i = \frac{1}{2}\sum_{i\neq j}\phi(r_{ij}(\rho_i)) \tag{S4}$$

where $\phi(r)$ is the pair potential given in eq. 1 of the main text and $r_{ij}(\rho_i)$ indicates all pair interactions positions at respective density $\rho_i$ drawn from the ground state radial distribution for each lattice $l_i$. The pressure is computed from the virial as

$$P_i = -\frac{1}{4}\rho_i\sum_{i\neq j} r_{ij}(\rho_i)\phi'(r_{ij}(\rho_i)) \tag{S5}$$

where $\phi'(r)$ indicates derivative with respect to $r$. These equations define the system physics and constitute the bulk of the non-linear problem solved in GAMS. In addition to those equations, we use the following auxiliary equations for each crystal to constrain the range of the possible $\rho_i$ as

$$r_c^2/d_0 > 1 \tag{S6}$$

where $r_c$ indicates the interaction cut-off radius, and $d_0$ the nearest neighbor distance for each $l_i$ at $\rho_i$. Finally, the objective function used to optimize the system is chosen to minimize the net free energy of the system i.e.

$$U_{\text{tot}} = (1-x)(U_2 - U_1) + U_1 \tag{S7}$$

In this manner, given some starting $\phi(r)$ interaction and a chosen pair $l_1, l_2$ (from a large set of combinations of common and specialized lattices), any binary mixture that lowers the free energy of the sytem $U_{\text{tot}}$ relative to a desired target is considered a competitor and added to the competitor pool for another target optimization iteration.

## IV. DERIVATION OF THE WELL MINIMUM POSITION UPDATE SCHEME FOR A SPLINE POTENTIAL

Consider a knot in the Akima spline whose position is denoted by $r_o$. Consider further a continuous functional representation of the spline at the $i$th iteration as $f_i$ with $r_o$ as a parameter, namely $f_i(r - r_o)$. Taking the derivative of $f_i$ with respect to $r$ we define a new function $g$ as

$$g_i(r - r_o) \equiv f_i'(r - r_o) \tag{S8}$$

Now suppose that the location of the well minimum for the current $i$th iteration is given by $r_o$. We can consider small changes around this minimum by doing a Taylor expansion on $g_i(r - r_o)$. Therefore

$$\begin{aligned} g_i(r - r_o) &= g_i(r_o) + g_i'(r_o)(r - r_o) + ... \\ g_i(r - r_o) &\approx m(r - r_o) \end{aligned} \tag{S9}$$

where for the last equation $g_i(r_o) = 0$ by definition and $m \equiv g_i'(r_o)$, denotes the slope of a line. Consider now the iteration $i+1$ where the Akima point freely changes by a small value $+\delta g$. From eq. S9 we then have approximately

$$g_{i+1}(r - r_o) \approx \delta g + m(r - r_o) \tag{S10}$$

and can determine the new minimum point $r_n$ by setting $g_{i+1}(r_n - r_o) = 0$. Using eq. S10 and solving for $r_n$ we get

$$r_n = r_o - \delta g/m \tag{S11}$$

In practice, we work with the negative difference of the Akima spline points for convinience i.e. $-g$. Therefore $m \equiv -m$ and eq. S11 becomes

$$r_n = r_o + \delta r \tag{S12}$$

where $\delta r \equiv \delta g/m$. A similar procedure for $-\delta g$ change in the akina knot at $r_o$ yields

$$r_n = r_o - \delta r \tag{S13}$$

Therefore, the update scheme is implemented as follows. If the Akima spline point $r_o$ which is also the minimum at the $i$th iteration changes by $+\delta g$ in the next iteration $i+1$, the new minimum position is defined as $\min(g_{i+1}(r_o), g_{i+1}(r_{o+1}))$ where $r_{o+1}$ indicates the spline

point immediately to the right of $r_o$ i.e. the point closest to 0 magnitude is defined as the new minimum for that iteration. The equivalent rule for $-\delta g$ is $\min(g_{i+1}(r_o), g_{i+1}(r_{o-1}))$, where $r_{o-1}$ indicates a spline point immidiately to the left of $r_o$.
